# Supplementary material for: Minimax-Optimal Predictive Flow Matching under Distribution Drift
Source: arXiv:2610.28898 source file (2026-10-20)
Supplement: Supplementary file 1 [file setup.tex]

\appendix
\renewcommand{\theequation}{\arabic{equation}}
\makeatletter
\setcounter{theorem}{0}\renewcommand{\thetheorem}{\thesection.\arabic{theorem}}\@addtoreset{theorem}{section}
\setcounter{lemma}{0}\renewcommand{\thelemma}{\thesection.\arabic{lemma}}\@addtoreset{lemma}{section}
\setcounter{proposition}{0}\renewcommand{\theproposition}{\thesection.\arabic{proposition}}\@addtoreset{proposition}{section}
\setcounter{corollary}{0}\renewcommand{\thecorollary}{\thesection.\arabic{corollary}}\@addtoreset{corollary}{section}
\setcounter{remark}{0}\renewcommand{\theremark}{\thesection.\arabic{remark}}\@addtoreset{remark}{section}
\setcounter{assumption}{0}\renewcommand{\theassumption}{\thesection.\arabic{assumption}}\@addtoreset{assumption}{section}
\makeatother
% ===== Original supplement.tex =====
\begin{center}
{\Large\bfseries Minimax-Optimal Predictive Flow Matching under Distribution Drift}\\[5pt]
{\large Supplementary Material}
\end{center}
